# Supplementary material for: Checkpoint Selection and Evaluation in EEG Emotion Recognition
Source: arXiv:2607.27655 source file (2026-09-14)
Supplement: Supplementary file 1 [file supplementary_information.tex]

% Supplementary Information appended to the arXiv preprint
\documentclass[pdflatex,sn-basic,Numbered]{sn-jnl}

\usepackage{amsmath,amssymb,amsfonts}
\usepackage{booktabs}
\usepackage{tabularx}
\usepackage{array}
\usepackage{microtype}
\usepackage{xurl}
\hypersetup{
  pdftitle={Supplementary Information for: Evaluation Protocols and Cross-Subject Generalization in EEG Emotion Recognition},
  pdfauthor={Hanting Suo; Yuwen Li},
  pdfsubject={Supplementary Information for the arXiv preprint}
}
\newcolumntype{Y}{>{\raggedright\arraybackslash}X}
\raggedbottom

\begin{document}

\title[Supplementary Information]{Supplementary Information for: Evaluation Protocols and Cross-Subject Generalization in EEG Emotion Recognition}
\author[1,2]{\fnm{Hanting} \sur{Suo}}
\author*[1,2]{\fnm{Yuwen} \sur{Li}}\email{liyuwen@seu.edu.cn}
\affil[1]{\orgdiv{School of Instrument Science and Engineering}, \orgname{Southeast University}, \orgaddress{\city{Nanjing}, \postcode{210096}, \country{China}}}
\affil[2]{\orgdiv{The State Key Laboratory of Bioelectronics}, \orgname{Southeast University}, \orgaddress{\city{Nanjing}, \postcode{210096}, \country{China}}}
\maketitle

\noindent\textbf{Journal submission:} Applied Intelligence\\
\textbf{Corresponding author:} Yuwen Li\\
\textbf{Corresponding author e-mail:} liyuwen@seu.edu.cn\\
\textbf{ORCID:} \href{https://orcid.org/0000-0003-3060-836X}{0000-0003-3060-836X}

This supplement reports the supporting analysis details moved from the main manuscript. It does not introduce new experiments or alter any pre-specified decision. All numerical values come from the same frozen results and independently audited artifacts used by the main text.

\clearpage
\section*{S1 Subject-level performance-ranking stability}

The reliability analysis was planned before inspection of its confirmatory outputs. It used all three sessions and all 15 participants in each public dataset. The primary representation was the official trial-level LDS differential-entropy vector summarized by its element-wise mean and standard deviation (\texttt{mean\_std}). A pre-specified sensitivity retained only the element-wise mean (\texttt{mean}). The sensitivity was diagnostic and could not replace a failed primary decision.

Classification was session-local and leave-one-subject-out. For each session and held-out participant, \texttt{StandardScaler} and an RBF SVM (\texttt{C=1.0}, \texttt{gamma="scale"}, \texttt{class\_weight="balanced"}) were fitted on the other 14 participants. Within each session and emotion class, sorted trial identifiers were assigned alternately to blocks A and B. The class-balanced trial partition was identical for every participant in that session. Accuracy was calculated for each block and the complete session. The three within-session comparisons correlated block-A and block-B accuracies across participants. The three cross-session comparisons correlated complete-session accuracies for sessions 1--2, 1--3, and 2--3.

Subject identities remained aligned. Conditional BCa intervals used 20,000 participant-level bootstrap draws with seed 20240713. Joint one-sided permutation tests used the same number of draws and seed. Split-half permutations applied one shared participant-label permutation to block-B values across the three sessions. Cross-session permutations fixed session 1 while independently permuting participant labels for sessions 2 and 3.

The primary SEED-IV hierarchy first required a split-half median Spearman correlation of at least 0.30. Persistent cross-session reliability then required a median of at least 0.40, joint \(p\leq0.05\), at least two positive pairwise correlations, and none at or below -0.20. SEED was a formal replication dataset only if primary SEED-IV passed. The 0.30 and 0.40 values were engineering stopping criteria fixed before the outputs. They are not significance cutoffs or general reliability categories.

\begin{table*}[!htbp]
\centering
\footnotesize
\setlength{\tabcolsep}{2.5pt}
\renewcommand{\arraystretch}{1.12}
\caption{Subject-level performance-ranking results. Pairwise values follow sessions 1, 2, and 3 for split-half comparisons and session pairs 1--2, 1--3, and 2--3 for cross-session comparisons. Intervals are conditional on the fitted models and fixed analysis panel.}\label{tab:S1}
\begin{tabularx}{\textwidth}{@{}YYYYYYY@{}}
\toprule
\textbf{Dataset and role} & \textbf{Summary} & \textbf{Contrast} & \textbf{Pairwise Spearman \(\rho\)} & \textbf{Median \(\rho\)} & \textbf{95\% BCa interval} & \textbf{Joint one-sided permutation \(p\)} \\
\midrule
SEED-IV primary & \texttt{mean\_std} & Split-half A vs B & -0.1436 / 0.5033 / 0.1700 & 0.1700 & [-0.2790, 0.5291] & 0.1696 \\
SEED-IV primary & \texttt{mean\_std} & Cross-session & 0.1037 / -0.3813 / 0.0470 & 0.0470 & [-0.1925, 0.5548] & 0.3757 \\
SEED-IV sensitivity & \texttt{mean} & Split-half A vs B & 0.5667 / 0.4770 / 0.7736 & 0.5667 & [0.1828, 0.7811] & 0.0012 \\
SEED-IV sensitivity & \texttt{mean} & Cross-session & -0.1732 / -0.0457 / 0.4934 & -0.0457 & [-0.5713, 0.4330] & 0.5628 \\
SEED diagnostic & \texttt{mean\_std} & Split-half A vs B & 0.5772 / 0.4594 / 0.5646 & 0.5646 & [0.2895, 0.7923] & 0.0011 \\
SEED diagnostic & \texttt{mean\_std} & Cross-session & -0.0766 / 0.2121 / 0.3376 & 0.2121 & [-0.2306, 0.6321] & 0.1076 \\
SEED diagnostic & \texttt{mean} & Split-half A vs B & 0.8646 / 0.5709 / 0.7736 & 0.7736 & [0.4688, 0.8998] & 0.00005 \\
SEED diagnostic & \texttt{mean} & Cross-session & 0.3300 / 0.4310 / 0.4503 & 0.4310 & [0.0059, 0.7861] & 0.0073 \\
\bottomrule
\end{tabularx}
\end{table*}

The primary SEED-IV criterion failed. The SEED rows therefore remain diagnostic even when their numerical criteria are favorable. The \texttt{mean} sensitivity establishes that within-session ranking can depend strongly on the feature summary; it does not rescue the lack of cross-session persistence on primary SEED-IV.

\clearpage
\section*{S2 SEED-IV implementation-consistency audit}

The local protocol-matched SEED-IV result was 0.4899, compared with the public reference value of 0.5239. The resulting difference of \(-0.0340\) exceeded the pre-specified two-percentage-point compatibility tolerance. We therefore performed a read-only audit of the exact local pathway without changing the protocol, tuning the model, or rerunning the scientific result.

The audit verified eight groups against the pinned LibEER source revision \texttt{39dc27e}. The selected released arrays were processed at 200 Hz with a 0.3--50 Hz pass band, five bands (0.5--4, 4--8, 8--14, 14--30, and 30--50 Hz), non-overlapping one-second segments, and differential entropy followed by LDS smoothing. The label table contained the SEED-IV four-class mapping \(0\)--\(3\) for 24 trials per recording; the three-class SEED mapping was not used. Raw-file order, first-sample removal, cache provenance, split construction, model settings, validation-based checkpoint selection, and subject-equal aggregation all matched the retained source and manifests.

\begin{table*}[!htbp]
\centering
\small
\setlength{\tabcolsep}{2.5pt}
\renewcommand{\arraystretch}{1.12}
\caption{Attribution audit for the SEED-IV protocol-matched compatibility difference. The eight verifiable groups passed; the final row records the boundary that prevented exact historical reproduction.}\label{tab:S2}
\begin{tabularx}{\textwidth}{@{}YYY@{}}
\toprule
\textbf{Audit group} & \textbf{Scope of verification} & \textbf{Outcome} \\
\midrule
Pinned source identity & Commit \texttt{39dc27e}; DGCNN source and configuration checksums & Passed \\
File and label tables & Three sessions, 15 participants per session, 24 trials per recording, four labels \(0\)--\(3\) & Passed \\
Raw-trial order and first-sample handling & Trial variables \texttt{eeg1}--\texttt{eeg24} in all 45 files; first sample removed by both loaders & Passed \\
Preprocessing-cache provenance & 200 Hz processing; 0.3--50 Hz filtering; five bands; one-second non-overlapping segments; source, shape, label, and dtype manifests & Passed \\
Preprocessing-function identity & Local wrapper called the pinned band-pass, differential-entropy, and LDS functions; unit-length segmentation preserved the generated windows & Passed \\
Trial-split equivalence & 270 direct pinned checks and 450 independent split-reconstruction checks & Passed \\
Model training and selection & 150 epochs, batch size 32, learning rate 0.001, upstream sampling, no added normalization, and earliest best validation macro-F1 & Passed \\
Aggregation and reference comparison & Subject-equal window accuracy 0.4899 versus 0.5239; difference \(-0.0340\) & Passed; tolerance not met \\
Historical public-run artifacts & Dependency lock, processed arrays, checkpoints, and unit predictions from the public reference run & Not available for verification \\
\bottomrule
\end{tabularx}
\end{table*}

None of the eight verifiable audit groups explained the 3.40-percentage-point difference. The unavailable historical artifacts prevent a claim of exact equivalence, so the difference remains unresolved. Accordingly, the strict SEED-IV result is retained only as a secondary sensitivity analysis and is not assigned the same evidential weight as the SEED result.

\clearpage
\section*{S3 Tail-risk ensemble development}

The tail-risk case used 555 engineered features: 310 differential-entropy features, 45 asymmetry features, 50 regional summaries, and 150 trial-context features. Seven components entered the mixture: three linear SVMs using DE-310, structural-245, or all-555 features; two RBF SVMs using DE-310 or all-555; XGBoost using all-555; and LightGBM using all-555. DGCNN and GCBNet were external comparators, not mixture components.

Linear SVM crossed \(C\in\{0.1,1,10\}\). RBF SVM crossed \(C\in\{1,10\}\) with \(\gamma\in\{\mathrm{scale},0.001\}\). XGBoost used either 200 trees, depth 3, and learning rate 0.05, or 400 trees, depth 2, and learning rate 0.03. LightGBM used either 200 trees, 15 leaves, and learning rate 0.05, or 400 trees, 31 leaves, and learning rate 0.03. Both boosting families used subsample and column-subsample rates of 0.9 and L2 regularization of 1.0. Candidates were ordered by validation window accuracy, macro-F1, and then the fixed grid order.

Complete-trial partitions were 9/3/3 train/validation/test trials per SEED subject-session and 16/4/4 for SEED-IV. For all 90 subject-session cells, sanitized development inputs retained only train and validation identifiers, split checksums, optimization seed, selected component parameters, validation labels and trial identifiers, and validation probabilities. Every JSON field or NPZ array whose key began with \texttt{test} was rejected. Three class-stratified complete-trial folds produced out-of-fold probabilities within the training trials. SVM calibration used two complete-trial folds inside each base fit.

For component probabilities \(p_{m,c}(x)\), weights \(w_m\geq0\), \(\sum_mw_m=1\), and \(\epsilon=10^{-6}\), the normalized mixture was

\[
\widetilde p_{w,c}(x)=
\frac{\max\{\epsilon,\sum_m w_m p_{m,c}(x)\}}
{\sum_{c'}\max\{\epsilon,\sum_m w_m p_{m,c'}(x)\}}.
\]

Let \(L_e(w)\) be mean multiclass log loss in environment \(e\), and let \(\mu(w)=E^{-1}\sum_eL_e(w)\). With \(\alpha\) as the VaR quantile, the implemented empirical upper-tail risk was

\[
\widehat{\mathrm{CVaR}}_\alpha(w)
=\min_{\eta}\left[
\eta+\frac{1}{(1-\alpha)E}
\sum_{e=1}^{E}\max\{L_e(w)-\eta,0\}
\right].
\]

The fitted tail configuration minimized

\[
(1-\lambda)\mu(w)+\lambda\widehat{\mathrm{CVaR}}_\alpha(w)
\quad\text{subject to}\quad
w\in\Delta_7,\qquad
\mu(w)\leq\min_m\mu(\mathbf e_m)+\delta.
\]

Tail candidates crossed \(\lambda\in\{0.25,0.5,0.75\}\), \(\alpha\in\{0.67,0.8\}\), and \(\delta\in\{0,0.01\}\). Mean-risk controls used \(\lambda=0\) with the same \(\delta\) values. SLSQP used \texttt{maxiter=2000}, \texttt{ftol=1e-10}, and constraint tolerance \texttt{1e-8}. Mean-risk and tail-risk candidates were selected separately by higher subject-equal validation accuracy, higher macro-F1, lower environment CVaR, smaller \(\lambda\), smaller \(\alpha\), and smaller \(\delta\). The strongest-single control minimized OOF-training mean environment log loss; uniform weights supplied the second direct control.

\begin{table*}[!htbp]
\centering
\small
\setlength{\tabcolsep}{2.5pt}
\renewcommand{\arraystretch}{1.12}
\caption{Selected mean-risk controls and tail-risk configurations. Displayed weights are rounded to six decimals; the machine-readable configuration file contains full precision. The stored \(\alpha\) is inert when \(\lambda=0\).}\label{tab:S3}
\begin{tabularx}{\textwidth}{@{}YYYYY@{}}
\toprule
\textbf{Parameter or component} & \textbf{SEED mean} & \textbf{SEED tail} & \textbf{SEED-IV mean} & \textbf{SEED-IV tail} \\
\midrule
\(\lambda\) & 0.00 & 0.75 & 0.00 & 0.25 \\
\(\alpha\) & 0.80 & 0.67 & 0.80 & 0.67 \\
\(\delta\) & 0.00 & 0.00 & 0.00 & 0.00 \\
Linear SVM, DE-310 & 0.285000 & 0.180849 & 0.335002 & 0.328846 \\
Linear SVM, structural-245 & 0.066939 & 0.104457 & 0.113510 & 0.143373 \\
Linear SVM, all-555 & 0.047778 & 0.036395 & 0.053116 & 0.051742 \\
RBF-SVM, DE-310 & 0.205927 & 0.253550 & 0.174831 & 0.151113 \\
RBF-SVM, all-555 & 0.047196 & 0.183455 & 0.064549 & 0.063961 \\
XGBoost, all-555 & 0.115313 & 0.115674 & 0.142294 & 0.131724 \\
LightGBM, all-555 & 0.231846 & 0.125620 & 0.116698 & 0.129241 \\
\bottomrule
\end{tabularx}
\end{table*}

Exact double-precision weights and the source checksum are also provided in \texttt{Supplementary material - CF-TRE final configurations.json}.

\clearpage
\section*{S4 Subject-dependent final controls}

The final comparison used the existing held-out trial partitions of the same 15 participants across three sessions. Selected ensemble weights were applied without further fitting. Primary accuracy was computed within each subject-session, averaged across sessions within participant, and then averaged equally across participants. This is a subject-dependent held-out-trial evaluation.

Logistic regression and random forest were added after advisor review. Both used the same 555 engineered features and final partitions as the ensemble. Logistic regression used training-only standardization, balanced class weights, \(C=1\), the \texttt{lbfgs} solver, and 2,000 maximum iterations. Random forest used 300 trees, the Gini criterion, square-root feature sampling, balanced class weights, and unrestricted depth. Neither model was tuned on validation or test outcomes. They remain post-review descriptive controls and cannot alter the original decision.

\begin{table*}[!htbp]
\centering
\small
\setlength{\tabcolsep}{2.5pt}
\renewcommand{\arraystretch}{1.12}
\caption{Subject-dependent final controls. Each cell reports subject-equal window accuracy / macro-F1.}\label{tab:S4}
\begin{tabularx}{\textwidth}{@{}YYYY@{}}
\toprule
\textbf{Method} & \textbf{SEED} & \textbf{SEED-IV} & \textbf{Role} \\
\midrule
Linear SVM, DE-310 & 0.7112 / 0.6796 & 0.5744 / 0.5156 & Pre-specified single-model control \\
Logistic regression, all-555 & 0.7265 / 0.6868 & 0.6148 / 0.5576 & Post-review descriptive control \\
Random forest, all-555 & 0.7003 / 0.6474 & 0.5572 / 0.4964 & Post-review descriptive control \\
Uniform mixture & 0.7330 / 0.6802 & 0.5789 / 0.5186 & Pre-specified fixed-weight control \\
Mean-risk mixture & 0.7522 / 0.7032 & 0.5781 / 0.5202 & Pre-specified objective control \\
Tail-risk mixture & 0.7476 / 0.7058 & 0.5783 / 0.5213 & Candidate method \\
DGCNN & 0.7283 / 0.6879 & 0.6576 / 0.6037 & Pre-specified deep comparator \\
GCBNet & 0.6857 / 0.6425 & 0.6339 / 0.5848 & Secondary deep comparator \\
\bottomrule
\end{tabularx}
\end{table*}

The classical mixture and DGCNN use different representations. These rows compare complete methods and do not isolate the effect of the tail-risk objective.

\clearpage
\section*{S5 Pre-specified decisions}

\begin{table*}[!htbp]
\centering
\small
\setlength{\tabcolsep}{2.5pt}
\renewcommand{\arraystretch}{1.12}
\caption{Decision outcomes and interpretation.}\label{tab:S5}
\begin{tabularx}{\textwidth}{@{}YYYYY@{}}
\toprule
\textbf{Study} & \textbf{Prospective question} & \textbf{Result} & \textbf{Decision} & \textbf{Interpretation} \\
\midrule
Competition four-cell decomposition & Is the DEP-target transfer penalty larger? & Differential penalty -0.065 [-0.117, -0.014] & Directional claim rejected & DEP target was descriptively harder within population; direction-specific transfer unsupported \\
Participant-ranking stability & Is rank stable enough for persistent weighting? & Primary split 0.1700, cross 0.0470; sensitivity split 0.5667, cross -0.0457 & Primary reliability criterion failed & Within-session rank was representation-sensitive; persistent cross-session group unsupported \\
Tail-risk development & Does the mixture beat development controls on both datasets? & Accuracy +0.0286 / +0.0510 & Development criteria passed & Eligible for one frozen final evaluation \\
Tail-risk final recognition & Does the mixture establish a gain over DGCNN? & +0.0193 [-0.0377, 0.0969] / -0.0794 [-0.1683, 0.0366] & Recognition criterion failed; further development stopped & Development success did not establish final recognition superiority \\
\bottomrule
\end{tabularx}
\end{table*}

The reported final intervals are conditional on the observed participants, fixed partitions, fitted models, training rules, and stated seeds. They do not include uncertainty from redrawing participants, rebuilding folds, retraining all models, or repeating model selection.

\section*{S6 Reproducibility boundary}

The supplement is descriptive of frozen artifacts rather than an independent replication. Exact configuration files, result ledgers, subject-level aggregates, and reconstruction reports are retained in the research workspace. The public repository at \href{https://github.com/hantingsuo/eeg-generalization-research}{https://github.com/hantingsuo/eeg-generalization-research} contains the analysis code, protocol implementations, audit scripts, tests, and machine-readable final configuration used for the public-data analyses. Competition data, labels, and derived participant-level predictions remain subject to the custodian's release conditions and are not included in the public package.

\end{document}
